# Supplementary material for: Does Code Quality Affect Pull Request Acceptance? An empirical study
Source: arXiv:1908.09321 source file (2019-08-25)
Supplement: Supplementary file 1 [file Appendix.tex]

\newpage

\label{Appendix}

\begin{table*}[]
\centering 
\section*{Appendix A}
\caption{Description of the Top-50 TD Items present in the Analyzed Pull Requests}
\label{tab:Description}
\begin{tabular}
{p{5.5cm}|p{0.9cm}|p{9.2cm}}
\hline 
\textbf{Rule ID}	& \textbf{Priority} &	\textbf{Description}	\\	\hline
AvoidBranchingStatementAsLastInLoop	& 2 &	Avoid using a branching statement as the last one in a loop.	\\	\hline
AvoidCatchingNPE & 3 &	Avoid catching a NullPointerException; consider removing the cause of the NPE.	\\	\hline
AvoidCatchingThrowable & 3 &	A catch statement should never catch a throwable since it includes errors.	\\	\hline
AvoidFieldNameMatchingMethodName & 3	&	Field capabilities have the same name as a method.	\\	\hline
AvoidReassigningParameters & 2	&	Avoid reassigning parameters in the code.	\\	\hline
AvoidUsingVolatile & 2	&	Use of volatile modifier is not recommended.	\\	\hline
BeanMembersShouldSerialize & 3	&	Non-transient, non-static member found. It needs to be marked as transient or needs to have accessors.	\\	\hline
ClassWithOnlyPrivateConstructorsShouldBeFinal & 1	&	A class that only has private constructors should be final.	\\	\hline
CollapsibleIfStatements & 3	&	Nested if statements could be combined.	\\	\hline
CompareObjectsWithEquals & 3	&	Use equals() to compare object references.	\\	\hline
ConstructorCallsOverridableMethod & 1	&	Overridable method called during object construction	\\	\hline
DefaultLabelNotLastInSwitchStmt & 3	&	The default label should be the last label in a switch statement.	\\	\hline
DontCallThreadRun & 4	&	Don't call Thread.run() explicitly, use Thread.start().	\\	\hline
DontImportSun & 4	&	Avoid importing anything from the sun.* packages.	\\	\hline
ExceptionAsFlowControl & 3	&	Avoid using exceptions as flow control.	\\	\hline
ExcessiveMethodLength & 3	&	Avoid really long methods.	\\	\hline
ExcessivePublicCount & 3	&	Class has too many public methods and attributes.	\\	\hline
FormalParameterNamingConventions & 1	&	The method parameter names do not match. '[a-z][a-zA-Z0-9]*'	\\	\hline
GenericsNaming & 4	&	Generics names should be one letter long and upper case.	\\	\hline
IdenticalCatchBranches & 3	&  Catch branch A is identical to branch B.	\\	\hline
JUnit4TestShouldUseTestAnnotation & 3	&	JUnit 4 tests that execute tests should use the @Test annotation; JUnit 5 tests should use @Test, @RepeatedTest, @TestFactory, @TestTemplate, or @ParameterizedTest.	\\	\hline
JUnitAssertionsShouldIncludeMessage & 3	&	JUnit assertions should include a message.	\\	\hline
JUnitTestContainsTooManyAsserts & 3	&	Unit tests should not contain more than 1 assert.	\\	\hline
JUnitTestsShouldIncludeAssert & 3	&	JUnit tests should include assert() or fail().	\\	\hline
LocalVariableNamingConventions & 1	&	The final local variable name does not match. '[a-z][a-zA-Z0-9]*'	\\	\hline
LongVariable & 3	&	Avoid excessively long variable names.	\\	\hline
LooseCoupling & 3	&	Avoid using certain implementation types like 'TreeSet'; the use of interfaces is preferred instead.	\\	\hline
MethodNamingConventions & 1	&	The JUnit 4 test method name does not match '[a-z][a-zA-Z0-9]*'.	\\	\hline
MethodReturnsInternalArray & 3	&	Method may expose an internal array in its return value.	\\	\hline
MissingBreakInSwitch & 3	&	A switch statement does not contain a break.	\\	\hline
MissingStaticMethodInNonInstantiatableClass & 3	&	Class cannot be instantiated and does not provide any static methods or fields.	\\	\hline
NonThreadSafeSingleton & 3	&	Singleton is not thread-safe.	\\	\hline
NullAssignment & 3	&	Assigning an object to null is a code smell.	\\	\hline
OneDeclarationPerLine & 4	&	One line for each declaration enhances code readability.	\\	\hline
OnlyOneReturn & 3	&	A method should have only one exit point, and that should be the last statement in the method.	\\	\hline
RedundantFieldInitializer & 3	&	Avoid using redundant field initializers.	\\	\hline
ReplaceVectorWithList & 3	&	Consider replacing Vector with the newer java.util.List.	\\	\hline
ShortInstantiation & 2	&	Avoid instantiating short objects. Call Short.valueOf() instead.	\\	\hline
SimplifiedTernary & 3	&	There are ternary operators that can be simplified using \|\| or \&\&.	\\	\hline
SimplifyBooleanAssertion & 3	&	assertTrue(!expr) can be replaced by assertFalse(expr).	\\	\hline
SingularField & 3 &	A class field could be replaced by a local variable.	\\	\hline
SuspiciousOctalEscape & 3	&	Suspicious decimal characters following octal escape in string literal	\\	\hline
SystemPrintln & 2	&	System.out.println is used.	\\	\hline
TooManyMethods & 3	&	A class has too many methods.	\\	\hline
UncommentedEmptyConstructor & 3	&	Empty constructor needs to be documented.	\\	\hline
UnconditionalIfStatement & 3	&	Do not use for statements that are always true or always false.	\\	\hline
UnnecessaryLocalBeforeReturn & 3	&	Consider simply returning the value vs. storing it in the local variable.	\\	\hline
UnnecessaryModifier & 3	&	Unnecessary modifier on a method: the method is already in a final class.	\\	\hline
UnusedImports & 4	&	Avoid unused imports	\\	\hline
UseAssertNullInsteadOfAssertTrue & 3	&	Use assertNull(x) instead of assertTrue(x==null), or assertNotNull(x) instead of assertFalse(x==null).	\\	\hline
UseConcurrentHashMap & 3	&	If you run Java5 or newer and have concurrent access, you should use the ConcurrentHashMap implementation.	\\	\hline
UseEqualsToCompareStrings & 3	&	Use equals() to compare strings instead of '==' or '!='.	\\	\hline
UseIndexOfChar & 3	&	String.indexOf(char) is faster than String.indexOf(String).	\\	\hline
UselessOverridingMethod & 3	&	Overriding method merely calls super.	\\	\hline
UselessStringValueOf & 3	&	No need to call String.valueOf to append to a string.	\\	\hline
UseVarargs & 4	&	Use varargs for methods or constructors that take an array as the last parameter.	\\	\hline
\end{tabular}
\end{table*}
